# Supplementary material for: Universal Operational Privacy in Distributed Quantum Sensing
Source: arXiv:2601.19206 ancillary file (2026-07-16)
Supplement: Supplementary file 1 [file supplemental_metarial.pdf]

# Supplemental Material for: Universal Operational Privacy in Distributed Quantum Sensing

Min Namkung,<sup>1,\*</sup> Dong-Hyun Kim,<sup>1,2,\*</sup> Seongjin Hong,<sup>2</sup> Yong-Su Kim,<sup>1,3</sup> Su-Yong Lee,<sup>4,5</sup> and Hyang-Tag Lim<sup>1,3,†</sup>

<sup>1</sup>*Center for Quantum Technology, Korea Institute of Science and Technology (KIST), Seoul 02792, Korea*

<sup>2</sup>*Department of Physics, Yonsei University, Seoul 03722, Korea*

<sup>3</sup>*Division of Quantum Information, KIST School,*

*Korea University of Science and Technology, Seoul 02792, Korea*

<sup>4</sup>*Emerging Science and Technology Directorate, Agency for Defense Development, Daejeon, 34186, Korea*

<sup>5</sup>*Weapon Systems Engineering, ADD School, University of Science and Technology, Daejeon, 34060, Korea*

(Dated: January 27, 2026)

---

\* These authors have contributed equally.

† hyangtag.lim@kist.re.kr

## I. THEORETICAL DETAILS

### A. Generalized universal privacy condition

Here we extend the universal operational privacy condition introduced in the main text to the case where clients estimate multiple global functions  $\mathbf{w}^{(1)\top}\phi, \dots, \mathbf{w}^{(r)\top}\phi$  simultaneously. The corresponding weight vectors  $\mathbf{w}^{(1)}, \dots, \mathbf{w}^{(r)} \in \mathbb{R}^m$  define a weight matrix  $\mathbf{W} = \sum_{j=1}^r \mathbf{w}^{(j)} \mathbf{w}^{(j)\top}$ . The generalized privacy quantifier is defined as

$$\mathcal{P}_{\mathbf{F}}(\mathbf{W}) = 1 - \frac{1}{r} \min_{\substack{\mathbf{v}^{(j)} \perp \mathbf{w}^{(j)} \\ \|\mathbf{v}^{(j)}\|_2=1}} \sum_{j=1}^r \mathbf{v}^{(j)\top} \mathbf{\Pi}_{\mathbf{F}} \mathbf{v}^{(j)}. \quad (\text{S1})$$

This definition consistently extends the operational interpretation of privacy discussed in the main text. If the classical Fisher information matrix (CFIM)  $\mathbf{F}$  is non-singular, the projector  $\mathbf{\Pi}_{\mathbf{F}}$  acts as the identity on the entire parameter space. In this case, each term  $\mathbf{v}^{(j)\top} \mathbf{\Pi}_{\mathbf{F}} \mathbf{v}^{(j)} = 1$ , leading to  $\mathcal{P}_{\mathbf{F}}(\mathbf{W}) = 0$  and indicating the absence of privacy.

By contrast, when  $\mathbf{F}$  is singular,  $\mathbf{\Pi}_{\mathbf{F}}$  projects onto a strict subspace of the parameter space. Consequently,  $\mathbf{v}^{(j)\top} \mathbf{\Pi}_{\mathbf{F}} \mathbf{v}^{(j)} < 1$  for all admissible vectors, yielding  $\mathcal{P}_{\mathbf{F}}(\mathbf{W}) > 0$ . Perfect privacy,  $\mathcal{P}_{\mathbf{F}}(\mathbf{W}) = 1$ , is achieved when all minimizing vectors  $\mathbf{v}^{(j)}$  lie entirely within the kernel of  $\mathbf{F}$ .

### B. Principle of no local parameter exposure

This subsection clarifies how the proposed privacy condition prevents the exposure of any individual local parameter, even when multiple global functions are estimated. We consider the estimation of the balanced global function  $\mathbf{w}^\top \phi = \phi_1 + \phi_2 + \dots + \phi_m$  with respect to  $\mathbf{w}_j = 1$ , as discussed in previous works [1–3]. Suppose that the kernel of the CFIM contains the vector  $\mathbf{v}_{\text{ker}} = [1, -1, 1, -1, \dots, 1, -1]$ .

For illustration, let  $m = 8$  and assume that the following four global functions can be estimated with vanishing variance:

$$\begin{aligned} \phi_1 + a\phi_2 + b\phi_3 + c\phi_4 + d(\phi_5 + \phi_6 + \phi_7 + \phi_8), \\ \phi_1 + e\phi_2 + f\phi_3 + g\phi_4 + h(\phi_5 + \phi_6 + \phi_7 + \phi_8), \\ \phi_1 + k\phi_2 + l\phi_3 + m\phi_4 + n(\phi_5 + \phi_6 + \phi_7 + \phi_8), \\ \phi_1 + p\phi_2 + q\phi_3 + r\phi_4 + s(\phi_5 + \phi_6 + \phi_7 + \phi_8), \end{aligned} \quad (\text{S2})$$

with nonzero coefficients.

If the coefficient matrix

$$\begin{bmatrix} 1 & 1 & 1 & 1 & 1 \\ 1 & a & b & c & d \\ 1 & e & f & g & h \\ 1 & k & l & m & n \\ 1 & p & q & r & s \end{bmatrix} \quad (\text{S3})$$

were invertible, the local parameters  $\phi_1, \phi_2, \phi_3$ , and  $\phi_4$  would be uniquely determined and thus exposed. However, orthogonality to the kernel vector  $\mathbf{v}_{\text{ker}}$  requires all weight vectors in Eq. (S2) to satisfy  $\mathbf{w}^{(j)} \perp \mathbf{v}_{\text{ker}}$  [4–6], which renders the columns of Eq. (S3) linearly dependent. As a result, no individual local parameter can be inferred, even though multiple global functions are estimated. This argument extends straightforwardly to an arbitrary number of parameters.

### C. Discussion for the case of $0 < \mathcal{P}_{\mathbf{F}}(\mathbf{w}) < 1$

We discuss the physical meaning of intermediate values of the privacy quantifier,  $0 < \mathcal{P}_{\mathbf{F}}(\mathbf{w}) < 1$ . Consider a CFIM whose support space has dimension  $(m - 1)$ , with the spectral decomposition

$$\mathbf{\Pi}_{\mathbf{F}} = \sum_{j=1}^{m-1} \mathbf{e}^{(j)} \mathbf{e}^{(j)\top}, \quad (\text{S4})$$

where  $\{e^{(j)}\}$  are orthonormal vectors and  $e^{(m)}$  spans the kernel of  $\mathbf{F}$ .

Let  $\mathbf{v}$  be a unit vector orthogonal to  $\mathbf{w}$ , expanded as  $\mathbf{v} = \sum_{j=1}^m c_j e^{(j)}$ . Then

$$\mathbf{v}^T \Pi_{\mathbf{F}} \mathbf{v} = |c_1|^2 + |c_2|^2 + \cdots + |c_{m-1}|^2, \quad (\text{S5})$$

If  $\mathbf{w}$  has a nonzero component along the kernel direction  $e^{(m)}$ , the minimizing vector  $\mathbf{v}$  necessarily overlaps with the support space, yielding  $\mathbf{v}^T \Pi_{\mathbf{F}} \mathbf{v} < 1$  and thus  $0 < \mathcal{P}_{\mathbf{F}}(\mathbf{w}) < 1$ .

Physically, the kernel direction splits the global function into two components:  $(\Pi_{\mathbf{F}} \mathbf{w})^T \phi$  and  $((e^{(m)} e^{(m)T}) \mathbf{w})^T \phi$ . Only the former can be estimated with finite precision [4–6], while the latter remains completely hidden. This regime therefore represents a geometric trade-off: privacy is guaranteed, but only the component of the global function supported by the CFIM can be accessed by the clients.

#### D. Verification of basis independence, continuity, and noise tolerance

##### 1. Basis independence

We verify that the universal privacy quantifier  $\mathcal{P}_{\mathbf{F}}(\mathbf{w})$  defined in the main text is invariant under changes of basis in the parameter space. Let  $\mathbf{O}$  be an orthogonal matrix implementing a basis transformation. Since  $\mathbf{O}$  preserves inner products, we have

$$\min_{\substack{\mathbf{v} \perp \mathbf{w}, \\ \|\mathbf{v}\|_2=1}} \mathbf{v}^T \Pi_{\mathbf{F}} \mathbf{v} = \min_{\substack{\mathbf{O}\mathbf{v} \perp \mathbf{O}\mathbf{w}, \\ \|\mathbf{O}\mathbf{v}\|_2=1}} (\mathbf{O}\mathbf{v})^T (\mathbf{O} \Pi_{\mathbf{F}} \mathbf{O}^T) (\mathbf{O}\mathbf{v}).$$

The projector  $\Pi_{\mathbf{O}\mathbf{F}\mathbf{O}^T}$  associated with the transformed CFIM  $\mathbf{O}\mathbf{F}\mathbf{O}^T$  is constructed from the rotated eigenvectors of  $\mathbf{F}$ , implying  $\mathcal{P}_{\mathbf{F}}(\mathbf{w}) = \mathcal{P}_{\mathbf{O}\mathbf{F}\mathbf{O}^T}(\mathbf{O}\mathbf{w})$ . Therefore, the privacy quantifier is basis independent.

##### 2. Continuity

We show that the privacy quantifier is continuous under small perturbations of the CFIM. Let  $\{e^{(j)}\}$  denote an orthonormal basis of eigenvectors spanning the support space of  $\mathbf{F}$ , and consider a perturbed CFIM  $\mathbf{F}(\epsilon)$  whose support is spanned by vectors  $e^{(j)} + \epsilon \mathbf{f}^{(j)}$ , where  $\epsilon \ll 1$  and  $\mathbf{f}^{(j)}$  represent small perturbations induced by experimental imperfections. The corresponding projector reads

$$\Pi_{\mathbf{F}(\epsilon)} = \sum_j \left( e^{(j)} + \epsilon \mathbf{f}^{(j)} \right)^T \left( e^{(j)} + \epsilon \mathbf{f}^{(j)} \right).$$

For any unit vector  $\mathbf{v}$ , we obtain

$$|\mathbf{v}^T \{ \Pi_{\mathbf{F}(\epsilon)} - \Pi_{\mathbf{F}} \} \mathbf{v}| \leq \epsilon A + \epsilon^2 B,$$

with finite coefficients  $A = 2 \left| \sum_j (\mathbf{v}^T e^{(j)}) (\mathbf{f}^{(j)T} \mathbf{v}) \right|$  and  $B = \left| \sum_j (\mathbf{v}^T \mathbf{f}^{(j)})^2 \right|$ . This establishes the continuity relation discussed in the main text.

##### 3. Noise tolerance

We show that perfect privacy,  $\mathcal{P}_{\mathbf{F}}(\mathbf{w}) = 1$ , is preserved under noisy channels. Any parameter-independent noise process transforms the encoded probe state into  $(1 - D)\hat{\rho}_{\phi} + D\hat{\sigma}$ , where  $\hat{\sigma}$  is independent of the parameters and  $D \in [0, 1]$  quantifies the noise strength. For a fixed measurement  $\mathcal{M}$ , the CFIM is convex in the state, yielding

$$\mathbf{v}^T \mathbf{F}((1 - D)\hat{\rho}_{\phi} + D\hat{\sigma}, \mathcal{M}) \mathbf{v} \leq (1 - D) \mathbf{v}^T \mathbf{F}(\hat{\rho}_{\phi}, \mathcal{M}) \mathbf{v},$$

where  $\mathbf{F}(\hat{\sigma}, \mathcal{M}) = 0$  since  $\hat{\sigma}$  carries no parameter information. If  $\mathcal{P}_{\mathbf{F}}(\mathbf{w}) = 1$ , there exists a direction  $\mathbf{v}$  in the kernel of  $\mathbf{F}$  such that  $\mathbf{v}^T \mathbf{F}(\hat{\rho}_{\phi}, \mathcal{M}) \mathbf{v} = 0$ . Consequently,

$$\mathbf{v}^T \mathbf{F}((1 - D)\hat{\rho}_{\phi} + D\hat{\sigma}, \mathcal{M}) \mathbf{v} = 0,$$

demonstrating that perfect privacy is preserved under parameter-independent noise.

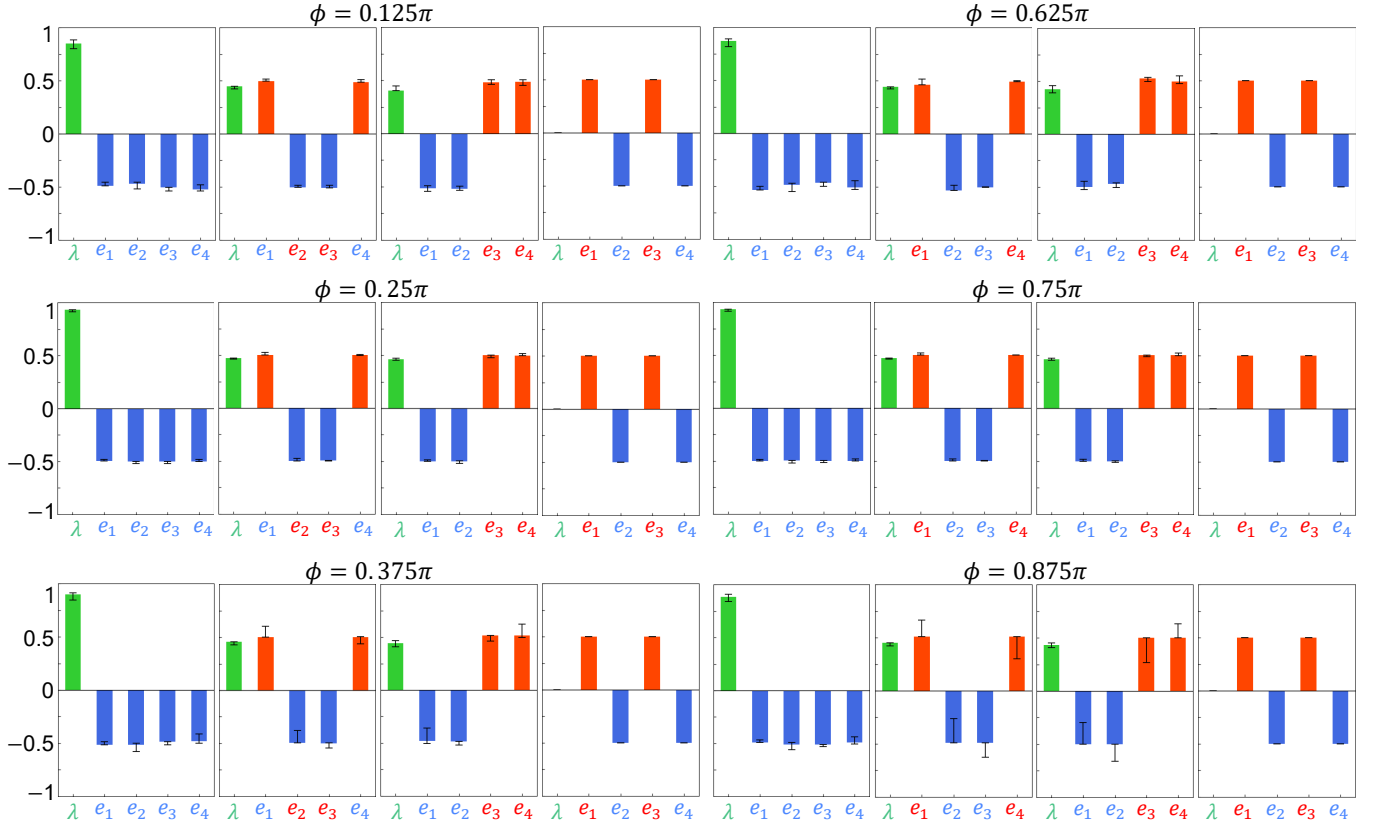

Supplementary Figure 1: Four eigenvalues and eigenvectors of the experimentally reconstructed CFIMs. The horizontal axis shows the eigenvalues  $\lambda$ , while the vertical axis displays the corresponding eigenvector components ( $e_1, e_2, e_3, e_4$ ). In the experiment, all phases are set to a common value  $\phi$ , i.e.,  $\phi_1 = \phi_2 = \phi_3 = \phi_4 = \phi$ . Error bars indicate the 95% confidence interval.

## II. EXPERIMENTAL DETAILS

Here we provide additional experimental details supporting the demonstration of private distributed quantum sensing for estimating the global function  $(\phi_1 + \phi_2 + \phi_3 + \phi_4)/4$ . Supplementary Fig. 1 presents the experimentally reconstructed CFIMs, including their four eigenvalues and corresponding eigenvectors.

As shown in Supplementary Fig. 1, the experimentally obtained CFIMs closely reproduce the theoretical CFIM, which has eigenvalues  $(1, 0.5, 0.5, 0)$  and corresponding eigenvectors  $(-0.5, -0.5, -0.5, -0.5)$ ,  $(-0.5, 0.5, 0.5, -0.5)$ ,  $(0.5, 0.5, -0.5, -0.5)$ , and  $(-0.5, 0.5, -0.5, 0.5)$  [7]. In particular, the presence of the eigenvector  $(-0.5, 0.5, -0.5, 0.5)$  associated with a zero eigenvalue confirms the singular structure of the CFIM realized in the experiment.

This experimentally verified kernel structure directly supports the privacy condition discussed in Supplementary Note I-B. Specifically, the existence of a kernel vector orthogonal to balanced global weight vectors implies that no information about any individual local phase is accessible to the untrusted servers. These observations confirm that the distributed quantum sensing network implemented in our experiment simultaneously achieves the desired global estimation task and the operational privacy guaranteed by the universal privacy condition.

- 
- [1] M. Hassani, M. Scheiner, M. G. A. Paris, and D. Markham, Privacy in networks of quantum sensors, *Phys. Rev. Lett.* **134**, 030802 (2025).
  - [2] L. Bugalho, M. Hassani, Y. Omar, and D. Markham, Private and robust states for distributed quantum sensing, *Quantum* **9**, 1596 (2025).
  - [3] A. de Oliveira Junior, A. L. Anderson, B. L. Larsen, S. W. Moore, D. Markham, M. Takeoka, J. B. Brask, and U. L. Anderson, Privacy in continuous-variable distributed quantum sensing, arXiv:2509.12338 (2025).

- [4] M. Namkung, C. Lee, and H.-T. Lim, Unified strategy for non-invertible Fisher information matrix in quantum metrology, *Phys. Lett. A* **564**, 131075 (2025).
- [5] P. Stoica and T. L. Marzetta, Parameter estimation problems with singular information matrices, *IEEE Trans. Signal Process.* **49**, 87 (2001).
- [6] Y.-H. Li and P.-C. Yeh, An interpretation of the Moore–Penrose generalized inverse of a singular Fisher information matrix, *IEEE Trans. Signal Process.* **60**, 5532–5536 (2012).
- [7] D.-H. Kim, S. Hong, Y.-S. Kim, Y. Kim, S.-W. Lee, R. C. Pooser, K. Oh, S.-Y. Lee, C. Lee, and H.-T. Lim, Distributed quantum sensing of multiple phases with fewer photons, *Nat. Commun.* **15**, 266 (2024).
